# Supplementary material for: Faster Optimization on Sparse Graphs via Neural Reparametrization
Source: arXiv:2205.13624 source file (2022-05-26)
Supplement: Supplementary file 1 [file scrap.tex]

\paragraph{Convergence Rate}
We will refer to $d\L/dt$ as the convergence rate, which for GF \eqref{eq:GF} is
\begin{align}
    {d\L\over dt}& = {\ro \L \over \ro \vw } \cdot {d\vw \over dt } = -\del \L ^T \eps \del \L 
    \label{eq:dLdt}
\end{align}
We will show how this rate gets modified by the reparametrization.

--------

% where with the Adam optimizer, $\hat{\eps}_{a} = \eta /
% \sqrt{\E[(\ro \L/\ro\theta_a)^2]+\xi} $
The convergence rate is then given by 
\begin{align}
    {d\L\over dt}& =\sum_{i,a} {\ro \L \over \ro \vw_i } {\ro \vw_i \over \ro \theta_a } {d\theta_a \over dt} \cr
    &= - \sum_{i,j}{\ro \L \over \ro \vw_i } {\ro \L \over \ro \vw_j} \sum_a \eps_a {\ro \vw_i \over \ro \theta_a}{\ro \vw_j \over \ro \theta_a} \cr
    &= - \sum_{i,j}M_{ij} K_{ij}
    = - \Tr\br{MK^T}, \\
    % K_{ij}& \equiv \sum_a {\ro \vw_i \over \ro \theta_a}{\ro \vw_j \over \ro \theta_a} \qquad M_{ij}\equiv {\ro \L \over \ro \vw_i } {\ro \L \over \ro \vw_j}
    % \qquad 
    K_{ij} &\equiv \sum_a \hat{\eps}_a {\ro \vw_i \over \ro \theta_a}{\ro \vw_j \over \ro \theta_a}.
    \label{eq:dLdt-Neural} 
    % \label{eq:dLdt-thm-MK}
    % \label{eq:NTK}
\end{align}
\out{
\begin{align}
    {d\L\over dt}& =\sum_{i,a} {\ro \L \over \ro \vw_i } {\ro \vw_i \over \ro \theta_a } {d\theta_a \over dt} = -\eps \sum_{i,j} {\ro \L \over \ro \vw_i } {\ro \L \over \ro \vw_j} \sum_a {\ro \vw_i \over \ro \theta_a}{\ro \vw_j \over \ro \theta_a} \cr
    &= -\eps \sum_{i,j}M_{ij} K_{ij}
    = -\eps \Tr\br{MK^T}, 
    \label{eq:dLdt-Neural} %\\
    % K_{ij}& \equiv \sum_a {\ro \vw_i \over \ro \theta_a}{\ro \vw_j \over \ro \theta_a} \qquad M_{ij}\equiv {\ro \L \over \ro \vw_i } {\ro \L \over \ro \vw_j}
    \qquad 
    K_{ij} \equiv \sum_a {\ro \vw_i \over \ro \theta_a}{\ro \vw_j \over \ro \theta_a}.
    % \label{eq:dLdt-thm-MK}
    % \label{eq:NTK}
\end{align}
}%%%%
% where $M_{ij}$ captures the gradients of $\L$ and $K_{ij}$ is the Neural Tangent Kernel (NTK) \citep{jacot2018neural}.
% \end{proof}
Here $K$ is the neural tangent kernel (NTK) \citep{jacot2018neural} of $\vw(\theta)$, and $M_{ij}$  is the squared gradients. 
Note, we have absorbed $\hat{\eps}_a$ into $K$ for convenience of notation. 

Define $\ba{M}=\E[M]$ and $\ba{K}=\E[K]$, the following theorem identifies the type of neural network architectures that can accelerate optimization through reparametrization
\begin{theorem}
With a neural reparametrization yielding $\br{\ba{K},\ba{M}}=0$,
to make all modes $\psi_i$ reach the ideal maximum rate $\max_i \|\psi_i^Td\vw/dt\|< \eta$, we need to have  
\begin{align}
    \ba{K} &\approx  %(M/m_{max})^{-1/2},
    \pa{{\ba{M}\over m_{max}}}^{-1/2}
    \label{eq:K-M-ideal}
\end{align}
% with $\max_i{k_i}=1$. 
\end{theorem}
\begin{proof}
This is because plugging $k_i^2 \approx m_{max} / (m_i+\xi) $ ($\xi\ll 1$) into \eqref{eq:psi-MK-commute} makes the r.h.s. equal to $\eta^2$.
% This means that, when $[\ba{K},\ba{M}]=0$, maximum speedup can be achieved if
\end{proof}

Next, we discuss how we can achieve this in practice. 
Specifically, we derive 
what architecture for the neural network $\vw(\theta)=f(\theta)$ will result in a $\ba{K}$ satisfying the condition in \eqref{eq:K-M-ideal}.

To find a neural network model that satisfies \eqref{eq:K-M-ideal}, we need to consider the fact that $\ba{M}(\vw(t))$ changes during optimization. 
To minimize the overhead from constructing $\vw(\theta)$ (and hence $\ba{K}$) as a function of $\ba{M}$, the architecture has to be as simple as possible and involve steps which do not increase the time complexity of each iteration significantly.

% We will now discuss when such neural reparametrization is feasible and how to implement \eqref{eq:K-M-ideal} in practice. 

\section{Neural Reparametrization}

% Using neural networks to reparametrize optimization problems  have been suggested in \citep{hoyer2019neural,sosnovik2019neural}. 

% \nd{We need a one page summary of results here. Maybe we can move the detailed derivations to the end of the paper and show the experiments before that?}
The high-level idea of neural reparametrization is that the optimization variable $\vw $ can be defined as the output of a  deep neural network $\vw(\theta) \equiv f(\theta)$ with trainable parameters $\theta$. 
Then, rather than optimizing over the original variables $\vw$ directly, we can instead optimize over the neural network parameters $\theta$. 
% Note that, in supervised settings the dataset $\mZ$ appeared in $\L(\vw;\mZ)$, which includes a loss function and a model architecture defining the model used. 
% The neural network $\vw(\theta)$ is a separate neural reparametrization of the trainable parameters in $\L(\vw;\mZ)$, which doesn't take the dataset $\mZ$ as explicit input. 
We  analyze gradient flow dynamics, which identifies the type of  neural network architectures that can accelerate the optimization. 

\subsection{Gradient Flow Dynamics}
All the problems discussed above can be formulated as  minimizing a smooth, lower-bounded loss function $\L(\vw)\in \R$ on abounded variable $\vw \in \R^n$:
\[\text{argmin}_{\vw} \L(\vw) \]
% 
% \ryu{can also be a matrix?}\nd{yes, $\vw$ can be a matrix. I discuss it below in lin reg.} For example a $p\times q$ weight matrix component $W_{ij}$ becomes $\vw_k$ with $k=c+i\cdot q + j $ (with $0\cdots c$ encoding other variables). 

When the optimization variables are matrices or tensors, $\vw$ represents a flattened vector containing all variables. $\vw$ can also represent all trainable parameters  in a deep neural network.
For supervised learning with   a dataset  $\mZ =\{(\V{x}_i, \V{y}_i)_{i=1}^N\}$, the loss function $\L(\vw)$ becomes $\L(\vw;\mZ)$. The dataset and the model class (e.g. architecture of a neural network) together define a loss landscape as a function of the optimization variables $\vw$. 
 
% \nd{this is general enough to include $\R^{n\times m}$, but we need to explain that later. } 
% is a high-dimensional vector of optimization parameters. 
% Many systems in physics and chemistry are of this nature. 
% For instance, $\L$ can be the free energy of a set of spins, as in the Ising model or Spin glasses \cite{bapst2020unveiling} \nd{cite}. 
% Note that these optimization problems do not involve an input dataset. 
% Additionally, the loss function is the energy function, determined by the properties of the system.
% \nd{Can we generalize to supervised problems?}
% \nd{I think these are ``Energy-based'' optimizations, to contrast from supervised or unsupervised, etc. learning which require a dataset. }
% We consider an optimization problem where we want to minimize a smooth, lower-bounded loss function $\L(\vw)$. 

% \subsection{Optimization as a Dynamical System}  are then defined via chain rule (backpropagation)
Gradient-based optimization updates the variables $\vw$ by taking repeated steps in the direction of the steepest descent $\vw^{t+1} = \vw^t -  \eps \frac{\ro \L}{\ro\vw^t}$ for a learning rate $\eps$. With very small time steps $\delta t$,  we examine the dynamics of $\vw(t)\in \R^n$ during the optimization process, treating $t$ as a continuous time. 
Using steepest descent for the optimization, $d\vw/dt$ follows the gradient flow:
\begin{align}
    {d\vw_i\over dt}& = -\eps_{ii} {\ro \L \over \ro \vw_i },
    \label{eq:GD}
\end{align}
where denote the learning rate $\eps $ as a diagonal matrix of learning rates.

\out{
It follows that after the 
% The immediate result of the 
``neural reparametrization'' 
the convergence rate can be expressed in terms of a Neural Tangent Kernel (NTK) \citep{jacot2018neural}:

\begin{proposition}[Rate of Loss Drop]
\label{prop:dLdt-TrMK-main} 
\ryu{we should specify the rate of acceleration}\nd{yes, we will talk about that too}
In the unsupervised optimization using GD with $\L(\vw)$ as above, 
using neural network $\vw(\theta) = f(\theta)$ to reparametrize the optimization variable $\vw$ yields 

\begin{align}
    {d\L(\vw(\theta))\over dt}&= -\eps \Tr\br{MK^T}, &
    K_{ij}& \equiv \sum_a {\ro \vw_i \over \ro \theta_a}{\ro \vw_j \over \ro \theta_a}
    \label{eq:dLdt-thm-MK}
\end{align}
where $K$ is the neural tangent kernel (NTK) of $\vw(\theta)$, and  squared gradients $M$ (\eqref{eq:dLdt-GD}). 
\end{proposition}
}%%%%
% \begin{proof}

\paragraph{Modified convergence rate}
Neural reparametrization of the variables $\vw(\theta)$  leads the following updating rule for $\theta$:
\begin{align}
    {d\theta_a \over dt} = -\hat{\eps}_{a} {\ro \L \over \ro \theta_a} = -\hat{\eps}_{a} \sum_i  {\ro \L \over \ro \vw_i } {\ro \vw_i \over \ro \theta_a} 
    \label{eq:d-theta-dt0}
\end{align}
% where with the Adam optimizer, $\hat{\eps}_{a} = \eta /
% \sqrt{\E[(\ro \L/\ro\theta_a)^2]+\xi} $
The convergence rate is then given by 
\begin{align}
    {d\L\over dt}& =\sum_{i,a} {\ro \L \over \ro \vw_i } {\ro \vw_i \over \ro \theta_a } {d\theta_a \over dt} \cr
    &= - \sum_{i,j}{\ro \L \over \ro \vw_i } {\ro \L \over \ro \vw_j} \sum_a \eps_a {\ro \vw_i \over \ro \theta_a}{\ro \vw_j \over \ro \theta_a} \cr
    &= - \sum_{i,j}M_{ij} K_{ij}
    = - \Tr\br{MK^T}, \\
    % K_{ij}& \equiv \sum_a {\ro \vw_i \over \ro \theta_a}{\ro \vw_j \over \ro \theta_a} \qquad M_{ij}\equiv {\ro \L \over \ro \vw_i } {\ro \L \over \ro \vw_j}
    % \qquad 
    K_{ij} &\equiv \sum_a \hat{\eps}_a {\ro \vw_i \over \ro \theta_a}{\ro \vw_j \over \ro \theta_a}.
    \label{eq:dLdt-Neural0} 
    % \label{eq:dLdt-thm-MK}
    % \label{eq:NTK}
\end{align}
\out{
\begin{align}
    {d\L\over dt}& =\sum_{i,a} {\ro \L \over \ro \vw_i } {\ro \vw_i \over \ro \theta_a } {d\theta_a \over dt} = -\eps \sum_{i,j} {\ro \L \over \ro \vw_i } {\ro \L \over \ro \vw_j} \sum_a {\ro \vw_i \over \ro \theta_a}{\ro \vw_j \over \ro \theta_a} \cr
    &= -\eps \sum_{i,j}M_{ij} K_{ij}
    = -\eps \Tr\br{MK^T}, 
    \label{eq:dLdt-Neural0} %\\
    % K_{ij}& \equiv \sum_a {\ro \vw_i \over \ro \theta_a}{\ro \vw_j \over \ro \theta_a} \qquad M_{ij}\equiv {\ro \L \over \ro \vw_i } {\ro \L \over \ro \vw_j}
    \qquad 
    K_{ij} \equiv \sum_a {\ro \vw_i \over \ro \theta_a}{\ro \vw_j \over \ro \theta_a}.
    % \label{eq:dLdt-thm-MK}
    % \label{eq:NTK}
\end{align}
}%%%%
% where $M_{ij}$ captures the gradients of $\L$ and $K_{ij}$ is the Neural Tangent Kernel (NTK) \citep{jacot2018neural}.
% \end{proof}
Here $K$ is the neural tangent kernel (NTK) \citep{jacot2018neural} of $\vw(\theta)$, and $M_{ij}$  is the squared gradients. 
Note, we have absorbed $\hat{\eps}_a$ into $K$ for convenience of notation. 

Define $\ba{M}=\E[M]$ and $\ba{K}=\E[K]$, the following theorem identifies the type of neural network architectures that can accelerate optimization through reparametrization
\begin{theorem}
With a neural reparametrization yielding $\br{\ba{K},\ba{M}}=0$,
to make all modes $\psi_i$ reach the ideal maximum rate $\max_i \|\psi_i^Td\vw/dt\|< \eta$, we need to have  
\begin{align}
    \ba{K} &\approx  %(M/m_{max})^{-1/2},
    \pa{{\ba{M}\over m_{max}}}^{-1/2}
    \label{eq:K-M-ideal}
\end{align}
% with $\max_i{k_i}=1$. 
\end{theorem}
\begin{proof}
This is because plugging $k_i^2 \approx m_{max} / (m_i+\xi) $ ($\xi\ll 1$) into \eqref{eq:psi-MK-commute} makes the r.h.s. equal to $\eta^2$.
% This means that, when $[\ba{K},\ba{M}]=0$, maximum speedup can be achieved if
\end{proof}

Next, we discuss how we can achieve this in practice. 
Specifically, we derive 
what architecture for the neural network $\vw(\theta)=f(\theta)$ will result in a $\ba{K}$ satisfying the condition in \eqref{eq:K-M-ideal}.

To find a neural network model that satisfies \eqref{eq:K-M-ideal}, we need to consider the fact that $\ba{M}(\vw(t))$ changes during optimization. 
To minimize the overhead from constructing $\vw(\theta)$ (and hence $\ba{K}$) as a function of $\ba{M}$, the architecture has to be as simple as possible and involve steps which do not increase the time complexity of each iteration significantly.

% We will now discuss when such neural reparametrization is feasible and how to implement \eqref{eq:K-M-ideal} in practice. 

\subsection{Efficient Implementation in Graph optimization problems \label{sec:implement} }

\paragraph{Relation to Hessian and Quasi-Newton}

\paragraph{Imeplentation Using GNN}

Because $\ba{M}$ may depend on $\vw(\theta)$, as in \eqref{eq:M-K-indep-constraint}, we need a $K$ that is independent of $\theta$ to ensure  $\E[MK]=\E[M]\E[K]$. 
The simplest architecture  is a linear model $\vw_i = \sum_a \kappa_{ia} \theta_a $, which yields 
$\ba{K} = \kappa \kappa^T \approx  (\ba{M}/m_{max})^{-1/2}$.
% Since we the $\psi_i$ with the smallest $m_i$ have the largest eigenvalues in $(\ba{M}/m_{max})^{-1/2}$, it may seem that the  $n\times q$ matrix $\kappa $ can be the $q$ principal components (PC) of $(\ba{M}/m_{max})^{-1/2}$. 
% However, this will not for our problem because according to \eqref{eq:psi-dw-theta-2} any $\psi_i$ that has eigenvalue zero in $\ba{K}$ will not evolve at all. 
We need $\ba{K}$ to be a full rank matrix, meaning that $\kappa$ needs to be at least $n\times n$. 
Since we need the least computationally expensive $\ba{K}$, we choose $\theta\in \R^n$, and let $\kappa$ be a symmetric $n\times n$ matrix. 
This way, $\kappa = \sqrt{\ba{K}} = (\ba{M}/m_{max})^{-1/4}$. 
For the initial stages, where $\ba{M} \approx \mathcal{H}^2/n$ we have $\kappa = \pa{\mathcal{H}/h_{max}}^{-1/2}$, with $\mathcal{H}$ being the Hessian. 

\paragraph{Relation to GCN}
% Evaluating this $\kappa$ may in practice be a challenge, which we will address next. 
% But before that, 
% let us interpret the constraints we have found so far on the architecture of the neural network. 
% We have $\vw = \kappa\theta$ where $\kappa = (M/m_{max})^{-1/4}$ is a matrix fixed by the loss function $\L$.
Since both $\theta \in \R^n$ and $\vw\in \R^n$, our linear $\vw = \kappa\theta$ architecture is essentially a Graph Convolutional Network (GCN) \citep{kipf2016semi} with the aggregation rule $\kappa = (\ba{M}/m_{max})^{-1/4}$, or a weighted adjacency matrix.
% Indeed, we can think of $\ba{M}$ as the weighted adjacency matrix for a graph with $n$ vertices (nodes) and $\theta $ and $\vw $ are node attributes. 
In fact, all of our derivations remain unchanged if $\vw\in \R^{n\times d}$ and $\theta \in \R^{n\times m}$ (i.e. if there are $d$ and $m$ features per node in $\vw $ and $\theta$). 
Thus, our claim is that we can speed up the optimization process by reparametrizing $\vw$ using a GCN with linear activation, as $\vw=\kappa \theta $, 
where $\theta$ are trainable and $\kappa$ is the aggregation function derived from the loss gradients.
However, evaluating this $\kappa$ during GD can be quite expensive ($O(n^3)$) for large $n$ (GD steps $\sim O(n^2)$). 
% As we discussed above, each step of GD may be $O(n^2)$ before neural reparametrization, while evaluating $\kappa$ is typically $O(n^3)$. 
% Even if we do not recalculate $\kappa $ at every step of GD, this is prohibitively expensive. 
Ideally we want an approximation for
% $(\ba{M}/m_{max})^{-1/4}$ 
$\kappa $ which is $O(qn^2)$ with $q\sim O(1)$.

\paragraph{Hybrid optimization}
To use \eqref{eq:K-M-ideal} at points other than the initial steps, we need to dynamically estimate and update $\ba{M}$. 
Though estimating $\ba{M}(t)$ efficiently with ideas from Adam is possible, in the current work we focus on the speeding up at early stages using \eqref{eq:M-Hessian2-short}.
Thus, our main proposal is to use a two stage hybrid optimization: 
1) use the Hessian to reparametrize $\vw(\theta)$ in early stages for some number of iterations and then 2) switch to the original optimization over $\vw$.

\paragraph{Per-step time complexity}
Since $\vw\in \R^n$, the complexity of computing $\L(\vw)$ is $O(np)$ where $p$ depends on the sparsity structure of $\L$. 
% For example if $\L \sim \|\vw\|^2$, $p \sim O(1)$, while if $\L \sim \vw^T L\vw $, we may have $p\sim O(n)$ when $L$ is a dense matrix. 
$\ba{M}$ is an $n\times n$ matrix and computing $\ba{M}^{-1/2}$ is $O(n^3)$ , which is very expensive when $n\gg 1$. 
The eigenvalue $m_{max}$ can be estimated iteratively in $O(qn^2)$. 
Hence, computing $\ba{K}$ by exactly following \eqref{eq:K-M-ideal} is not feasible, unless $\ba{M}$ is fixed and can be calculated offline. 
Even then, evaluating $\ba{M}^{-1/2}$ only makes sense if the expected GD steps for convergence is more than $O(n)$, otherwise we don't gain any speedup.  
We may instead try to approximate $M^{-1/2}$ and $m_{max}$ iteratively with complexity $O(qn^2)$ where $q\ll n$ is the number of iterations. 
Hence we note that using \eqref{eq:K-M-ideal} to speedup the optimization may generally be useful if the the per step complexity of GD on $\L$ has a time complexity of least $O(qn^2)$.
\begin{figure}[t!]
 \centering
 % a\hfill b\hfill c\hfill .
 \includegraphics[width=\linewidth]{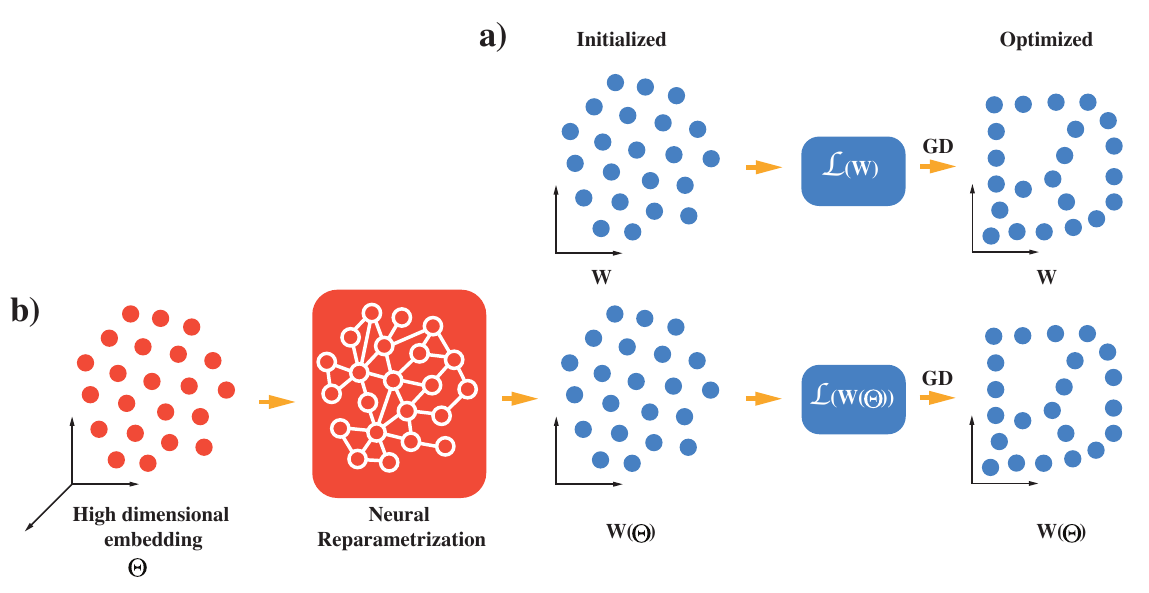}
 % trim=0 0 0 .5in, clip
%  ]{figures/reparam-model-2.pdf}
 \caption{Original (a) vs Neural Reparametrization (b) of the optimization problem. }
 \label{fig:model-reparam}
\end{figure}

\paragraph{Computationally efficient implementation} 
% \ry{how is this different from earlier paragraphs?}
We will focus on speeding up the early stages, in which we use the Hessian $\mathcal{H}$ in $\ba{M} \approx \mathcal{H}^2/n$. 
Define $\mH\equiv (1-\xi)\mathcal{H}/h_{max}$, where $h_{max}=\sqrt{m_{max}}$ and $\xi\ll 1$. 
To get an $O(qn^2)$ approximation for $\kappa = (\ba{M}/m_{max})^{-1/4}=\mH^{-1/2}$ we can take the first $q$ terms in the binomial expansion (see Appendix \ref{ap:implement}). 
A rough estimate would be 
\begin{align}
    \mH^{-1/2} &\approx I- {1\over 2} (I-\mH) -{3\over 4} (I-\mH)^2.
    \label{eq:M14-rough}
\end{align}
Since $\mH$ is positive semi-definite and its largest eigenvalue is $1-\xi <1 $, the sum in \eqref{eq:M14-rough} can be truncated after $q\sim O(1)$ terms. 
% \nd{should we change to $M/(m_{max}+\xi)$ for a small $\xi\ll1$ to argue for truncating the sum? (since technically we need all eigenvalues smaller than 1)}
The first $q$ terms of 
\eqref{eq:M14-expand} can be implemented as a $q$ layer GCN with aggregation function $f(\ba{M}) = I-M_0$ and residual connections.
We choose $q$ to be as small as $1$ or $2$, as larger $q$ may actually slow down the optimization. 
% \nd{move following to appendix?}
Note that computing $f(M_0)^q\theta $ is $O(qn^2)$ because we do not need to first compute $f(\ba{M})^q$ (which is $O(qn^3)$) and instead use $\vv_{i+1}f(\ba{M})\vv_i$ ($O(n^2)$) $q$ times with $\vv_1 = \theta$. 
% \nd{discuss architecture details.}

Lastly, to evaluate $M_0$ we need to estimate the leading eigenvalue $m_{max}$. 
% % \nd{Since $1/4$ is much smaller than one, $\prod_{i=0}^m(-1/4-i) \approx (-1)^m m!$ and we can further simplify?} 
% We can use a similar expansion for approximating $m_{max}$. 
Given any vector $\vv \in \R^n$ and using  spectral expansion, we have 
\begin{align}
    \mathcal{H}^q \vv &= \sum_i m_i^{q/2}  (\psi_i^T \vv)\psi_i & \Rightarrow &
    & 
    % m_{max}^{p-1} &\approx \frac{\mathbf{1}^T M^p \mathbf{1}}{\mathbf{1}^T M \mathbf{1}}
    h_{max} \approx \frac{\mathbf{1}^T\mathcal{H}^2 \mathbf{1}}{\mathbf{1}^T \mathcal{H} \mathbf{1}} = \frac{\sum_{ij} \mathcal{H}_{ij}^2}{\sum_{ij} \mathcal{H}_{ij}} 
    \label{eq:m-max-approx-D2-0}
\end{align}
where, since $\mathcal{H}$ is positive semi-definite, for $q>1$ the leading eigenvector $\psi_{max}$ quickly dominates the sum and we have $\mathcal{H}^q \vv \approx h_{max}^q (\psi_{max}\vv)\psi_{max} $.
Here we chose $q=2$ to get a crude approximation for $h_{max}$. 
The generalized Perron-Frobenius theorem \citep{berman1994nonnegative}, state the components of the leading eigenvector $\psi_{max}$ should be mostly positive. 
Therefore, we chose $\vv = \mathbf{1}/\sqrt{n}$, where $\mathbf{1}= (1,\dots, 1)$, which should be close to the actual $\psi_{max}$.

If we think of $M$ as the weighted adjacency matrix of a graph with $n$ vertices, the vector component $D_i = [\mathcal{H}\mathbf{1}]_i= \sum_j\mathcal{H}_{ij} $ is the weighted degree of node $i$.
Hence \eqref{eq:m-max-approx-D2-0} states $\mathcal{H}/m_{max} \approx\pa{\sum_i D_i/ \|D\|^2} \mathcal{H} $. 
This is similar to the graph diffusion operator $D^{-1} \mathcal{H} $ and $D^{-1/2}\mathcal{H} D^{-1/2}$ which are used as the aggregation functions in GCN (here $D_{ij} = D_i \delta_{ij}$ is the degree matrix).

% \paragraph{Final implementation}$\eps_i\sim \eta/\sqrt{\E[\mathrm{diag}(MK)]+\xi}$
When using modern optimizers, the adaptove learning rates  is a term within $\ba{K}$.
This will interfere with the optimal choice for $\kappa$ and hence our GCN aggregation function. 
Therefore, in practice, we do not fix the coefficients for $\mathcal{H}$ and $\mathcal{H}^2$ in our GCN. 
Instead, we use single or two layer GCN with aggregation function $f(\mathcal{H} )=D^{-1/2}\mathcal{H} D^{-1/2}$. 

\out{
This is a crude approximation, but it serves our goal by being computationally efficient. 
Note that, while computing $M^q$ is $O(qn^3)$, because $M\mathbf{1}$ is $O(n^2)$, computing $M^q\mathbf{1}$ is $O(qn^2)$.  
\nd{Todo: Check if $[M,K]=0$ yields maximum speedup.}
}%%%

Using \eqref{eq:GD}, we can derive the expected convergence rate over a time interval $[t-\Delta t, t]$ as follows. 
Define the convergence rate as the rate of change of the loss $d\L/dt$. 
Defining the gradient $g_t = \del \L(\vw(t)) $ and  using \eqref{eq:GD} we have
\begin{align}
    {d\L\over dt}& = {\ro \L\over \ro \vw}\cdot {d\vw \over dt} = -\eps \|g_t\|^2
\end{align}
where the $\cdot $ sums over all components of $\vw$. 
The expected value $\E_{\Delta t}$ over $[t,t+\Delta t]$ is given by 
\begin{align}
    \E_{\Delta t}\br{{d\L\over dt}}& = {1\over \Delta t} \int_t^{t+\Delta t} ds {d\L(\vw(s))\over ds} \cr 
    &= \int_t^{t+\Delta t} ds \|g_s\|^2 
    % \cr &
    = \Tr\br{G(t)}\cr 
    G(t) &\equiv \int_t^{t+\Delta t} ds g_sg_s^T 
\end{align}
where $G(t)$ is a symmetric quadratic matrix constructed from gradients $g_t$ over the $[t,t+\Delta t]$ interval.
The spectral properties of $G_t$ determine the rate of change of $\vw$ in different directions and are the foundation of most adaptive gradient optimizers, such as AdaGrad \citep{duchi2011adaptive}. 
Building on the results presented in \cite{duchi2011adaptive},
the idea of these optimizers is to speed up directions where the gradients are smaller.  This is achieved by making the learning rate $\eps \approx  \eta G_t^{-1/2} $  a preconditioning matrix \citep{duchi2011adaptive}, which in gradient flow notation yields
\begin{align}
    {d\vw_i\over dt}& = -\eta G_t^{-1/2} {\ro \L \over \ro \vw_i },
    \label{eq:GD-optimal-adagrad}
\end{align}
However, computing the inverse square root of a large matrix $G_t$ of parameter gradients is thought to be not feasible. 
There Adagrad, Adam, and most other optimizers approximate \eqref{eq:GD-optimal-adagrad} by using a diagonal version $\mathrm{diag}(G_t)$ instead of $G_t$. 
More recently, Shampoo \cite{gupta2018shampoo,anil2020scalable} has generalized this slightly by working with an approximation of $G_t$ sparsified in a certain way. 
Shampoo organizes the parameters $\vw$ into weights of different layers \nd{write about the matrix left and right gradients used in Shampoo. Review Anil et al more recent paper.
Propose experiments.}
The goal of the preconditioner is to make the dynamics of $\vw$ isotropic along all $\psi_i$, thereby making all directions evolve at the maximum rate that would be numerically stable. 
To see this, denote its eigendecomposition by $G_t =\sum_i \lambda_i \psi_i \psi_i^T $.  
Assuming the For the rate of change of $\vw$ along $\psi_i(t)$ we have

The eigenvalues $\lambda_i$ determine the expected rate of convergence of $\vw$ along eigenvector $\psi_i$. 
More generally, $\eps$ can be a matrix. 

where denote the learning rate $\eps $ as a diagonal matrix of learning rates.

% \section{Improving Convergence Rates Using Adaptive Gradient Methods}

\out{
It follows that after the 
% The immediate result of the 
``neural reparametrization'' 
the convergence rate can be expressed in terms of a Neural Tangent Kernel (NTK) \citep{jacot2018neural}:

\begin{proposition}[Rate of Loss Drop]
\label{prop:dLdt-TrMK-main} 
\ryu{we should specify the rate of acceleration}\nd{yes, we will talk about that too}
In the unsupervised optimization using GD with $\L(\vw)$ as above, 
using neural network $\vw(\theta) = f(\theta)$ to reparametrize the optimization variable $\vw$ yields 

\begin{align}
    {d\L(\vw(\theta))\over dt}&= -\eps \Tr\br{MK^T}, &
    K_{ij}& \equiv \sum_a {\ro \vw_i \over \ro \theta_a}{\ro \vw_j \over \ro \theta_a}
    \label{eq:dLdt-thm-MK}
\end{align}
where $K$ is the neural tangent kernel (NTK) of $\vw(\theta)$, and  squared gradients $M$ (\eqref{eq:dLdt-GD}). 
\end{proposition}
}%%%%
% \begin{proof}

\subsection{Efficient Implementation with GNN \label{ap:implement} }

Because $\ba{M}$ may depend on $\vw(\theta)$, as in \eqref{eq:M-K-indep-constraint},  we need a $K$ that is independent of $\theta$ to ensure  $\E[MK]=\E[M]\E[K]$. 
The simplest architecture  is a linear model $\vw_i = \sum_a \kappa_{ia} \theta_a $, which yields 
$\ba{K} = \kappa \kappa^T \approx  (\ba{M}/m_{max})^{-1/2}$.
% Since we the $\psi_i$ with the smallest $m_i$ have the largest eigenvalues in $(\ba{M}/m_{max})^{-1/2}$, it may seem that the  $n\times q$ matrix $\kappa $ can be the $q$ principal components (PC) of $(\ba{M}/m_{max})^{-1/2}$. 
% However, this will not for our problem because according to \eqref{eq:psi-dw-theta-2} any $\psi_i$ that has eigenvalue zero in $\ba{K}$ will not evolve at all. 
We need $\ba{K}$ to be a full rank matrix, meaning that $\kappa$ needs to be at least $n\times n$. 
Since we need the least computationally expensive $\ba{K}$, we choose $\theta\in \R^n$, and let $\kappa$ be a symmetric $n\times n$ matrix. 
This way, $\kappa = \sqrt{\ba{K}} = (\ba{M}/m_{max})^{-1/4}$. 
For the initial stages, where $\ba{M} \approx \mathcal{H}^2/n$ we have $\kappa = \pa{\mathcal{H}/h_{max}}^{-1/2}$, with $\mathcal{H}$ being the Hessian. 

\paragraph{Relation to GCN}
% Evaluating this $\kappa$ may in practice be a challenge, which we will address next. 
% But before that, 
% let us interpret the constraints we have found so far on the architecture of the neural network. 
% We have $\vw = \kappa\theta$ where $\kappa = (M/m_{max})^{-1/4}$ is a matrix fixed by the loss function $\L$.
Since both $\theta \in \R^n$ and $\vw\in \R^n$, our linear $\vw = \kappa\theta$ architecture is essentially a Graph Convolutional Network (GCN) \citep{kipf2016semi} with the aggregation rule $\kappa = (\ba{M}/m_{max})^{-1/4}$, or a weighted adjacency matrix.
% Indeed, we can think of $\ba{M}$ as the weighted adjacency matrix for a graph with $n$ vertices (nodes) and $\theta $ and $\vw $ are node attributes. 
In fact, all of our derivations remain unchanged if $\vw\in \R^{n\times d}$ and $\theta \in \R^{n\times m}$ (i.e. if there are $d$ and $m$ features per node in $\vw $ and $\theta$). 
Thus, our claim is that we can speed up the optimization process by reparametrizing $\vw$ using a GCN with linear activation, as $\vw=\kappa \theta $, 
where $\theta$ are trainable and $\kappa$ is the aggregation function derived from the loss gradients.
However, evaluating this $\kappa$ during GD can be quite expensive ($O(n^3)$) for large $n$ (GD steps $\sim O(n^2)$). 
% As we discussed above, each step of GD may be $O(n^2)$ before neural reparametrization, while evaluating $\kappa$ is typically $O(n^3)$. 
% Even if we do not recalculate $\kappa $ at every step of GD, this is prohibitively expensive. 
Ideally we want an approximation for
% $(\ba{M}/m_{max})^{-1/4}$ 
$\kappa $ which is $O(qn^2)$ with $q\sim O(1)$.

\paragraph{Hybrid optimization}
To use \eqref{eq:K-M-ideal} at points other than the initial steps, we need to dynamically estimate and update $\ba{M}$. 
Though estimating $\ba{M}(t)$ efficiently with ideas from Adam is possible, in the current work we focus on the speeding up at early stages using \eqref{eq:M-Hessian2-short}.
Thus, our main proposal is to use a two stage hybrid optimization: 
1) use the Hessian to reparametrize $\vw(\theta)$ in early stages for some number of iterations and then 2) switch to the original optimization over $\vw$.

\paragraph{Per-step time complexity}
Since $\vw\in \R^n$, the complexity of computing $\L(\vw)$ is $O(np)$ where $p$ depends on the sparsity structure of $\L$. 
% For example if $\L \sim \|\vw\|^2$, $p \sim O(1)$, while if $\L \sim \vw^T L\vw $, we may have $p\sim O(n)$ when $L$ is a dense matrix. 
$\ba{M}$ is an $n\times n$ matrix and computing $\ba{M}^{-1/2}$ is $O(n^3)$ , which is very expensive when $n\gg 1$. 
The eigenvalue $m_{max}$ can be estimated iteratively in $O(qn^2)$. 
Hence, computing $\ba{K}$ by exactly following \eqref{eq:K-M-ideal} is not feasible, unless $\ba{M}$ is fixed and can be calculated offline. 
Even then, evaluating $\ba{M}^{-1/2}$ only makes sense if the expected GD steps for convergence is more than $O(n)$, otherwise we don't gain any speedup.  
We may instead try to approximate $M^{-1/2}$ and $m_{max}$ iteratively with complexity $O(qn^2)$ where $q\ll n$ is the number of iterations. 
Hence we note that using \eqref{eq:K-M-ideal} to speedup the optimization may generally be useful if the the per step complexity of GD on $\L$ has a time complexity of least $O(qn^2)$.

\section{Theory}

Modern optimizers such as RMSProp \citep{tieleman2012lecture} or Adam \citep{kingma2014adam} choose $\eps$ adaptively for each $\vw_i$.
Specifically, in Adam and RMSProp \csb{we need to show experimental results by using both optimizers}, which we use in experiments, we have 
\begin{align}
    \eps_{ij}(\del \L,t) &\approx  {\eta \over \sqrt{\E_t[(\del_i \L)^2]} +\xi } \delta_{ij}
    \label{eq:Adam-eps}
\end{align}
where $\delta_{ij}$ is the Kronecker delta, and $\eta$  and $\xi$ are small numbers.
The expected value $\E$ is calculated using stochastic samples for $\del_i\L$ over multiple iteration steps, with more weights given to more recent steps.  
\Eqref{eq:GD} is also an ordinary differential equation (ODE). 
The local minima of $\L(\vw)$ correspond to the stationary solutions of the ODE, i.e. $d\vw/dt = 0$.

\paragraph{Convergence rate}
We are interested in the expected convergence rate $\E[d\L/dt]$ of the loss function. 
This expectation can be either approximated in a fashion similar to adaptive gradient optimizers (i.e. exponential time average) or be over random initializations under a distribution  $P(\vw(0))$. 
We will assume the expectation value for $\eps$ and $\E[d\L/dt]$ are evaluated with the same method, meaning we assume $\E[\eps]= \eps$. 
The convergence rate is then given by
\begin{align}
    \E\br{{d\L(\vw)\over dt}}& = \E\br{ \sum_i {\ro \L \over \ro \vw_i } {d\vw_i \over dt}} %= -\eps \E\br{\left\|{\ro \L \over \ro \vw }\right\|^2} 
    =- \Tr\br{\eps \ba{M}},
    % \label{eq:dLdt-GD} 
    & \\
    \ba{M}_{ij}&\equiv \E\br{ {\ro \L \over \ro \vw_i } {\ro \L \over \ro \vw_j}}
    % \label{eq:M-grad}
    \label{eq:dLdt-expect}
\end{align}
where we used our assumption to get $\E[\eps M] = \eps\E[M]$, with $M_{ij}=\del_i \L \del_j \L$ being the ``square gradients'' matrix  and $\ba{M}=\E[M]$.
With this definition, \eqref{eq:Adam-eps} becomes $\eps = \eta / \sqrt{\mathrm{diag}[\ba{M}] + \xi} $. 
\out{
\begin{align}
    \E\br{{d\L(\vw)\over dt}}& = \E\br{ \sum_i {\ro \L \over \ro \vw_i } {d\vw_i \over dt}} = -\eps \E\br{\left\|{\ro \L \over \ro \vw }\right\|^2} 
    =-\eps \Tr[M],
    % \label{eq:dLdt-GD} 
    &
    \bar{M}_{ij}&\equiv \E\br{ {\ro \L \over \ro \vw_i } {\ro \L \over \ro \vw_j}}
    % \label{eq:M-grad}
    \label{eq:dLdt-expect}
\end{align}
}%%%%%%
% where the ``squared gradients'' matrix $M$ %, encodes the gradients of $\L$ with respect to $\vw(t)$. 
Note that $\ba{M}$ 
is time-dependent and can change during optimization. 
% \nd{reword} need to estimate how long it would take the system to get close to a local minimum. 
% Note that for a given initialization $\vw(0)$, the gradient $\del \L= \ro\L/\ro \vw \in \R^n $ is a vector and the matrix $M$ is rank $1$, with its sole nonzero eigenvalue being $\|\del \L\|$ with eigenvector $\del \L /\|\del \L\|$.
%  Therefore, to estimate $d\L/dt$ in a typical case we treat the initialization $\vw(0)$ as an instance of a random variable and take the expected values. 

\paragraph{Estimating $\ba{M}$}
If we know the distribution $P(\vw(t))$ for some $t$, we can approximate $\ba{M}$. 
One way to do this is similar to Adam as a weighted average over the past few steps. 
% But in some problems there is no input dataset, such as the energy minimization problems we use in our experiments, and therefore there is no stochasticity.
Also, if we know the distribution of the initialization $P(\vw(0))$, we can evaluate $\ba{M}$ for early stages, which is what we will use in the current paper. 
When using Xavier initialization \citep{glorot2010understanding}, we have $\vw(0)\sim \mathcal{N}(0,n^{-1/2}) $.
In this case we can show (see appendix \ref{ap:M-estimate})
\begin{align}
    \ba{M}_{ij}(t\to 0)& =\sum_{k,l} \E[\vw_k\vw_l] {\ro^2 \L \over \ro \vw_k\ro \vw_i } {\ro^2 \L \over \ro \vw_l\ro \vw_j } + O(n^{-2}) \\
    %= {1\over n} \br{\mathcal{H}^2(\vw \to 0)}_{ij} +
    &= {1\over n}\left.\br{\mathcal{H}^2}_{ij}\right|_{\vw \to 0} + O(n^{-2}), 
    \label{eq:M-Hessian2-short}
\end{align}
where $\mathcal{H}_{ij}(\vw)\equiv \ro^2 \L(\vw)/\ro \vw_i \ro \vw_j$ is the Hessian of the loss at $t=0$.  

The eigenvectors of $\ba{M}$ with zero eigenvalue  are modes that do not evolve during optimization.
As gradients are zero in these directions, GD can never find and explore those directions. 
Therefore, we may exclude them from the beginning and claim that $\ba{M}$ is full rank. 

The rate $d\vw_i/dt$ can be different along different directions of the parameter space, with fast and slow modes.  Next, we quantify this difference in rates and suggest ways for acceleration.

\subsection{Computationally efficient implementation\label{ap:implement}}

Define $M_0\equiv (1-\xi)M/m_{max}$ with $\xi\ll 1$. 
To get an $O(qn^2)$ approximation for $\kappa = M_0^{-1/4}$ we can take the first $q$ terms in the binomial expansion
\begin{align}
    M_0^{-1/4} &= \br{ I+(M_0-I)}^{-1/4} \\
    % =\sum_{m=0}^\infty {(-1/2)\cdots(-1/2-m)\over m!} (M-I)^m 
    =\sum_{m=0}^\infty {\prod_{i=0}^m(-1/4-i)\over m!} (M_0-I)^m
    % \approx {-1\over 4} \sum_{m=0}^\infty (I-M_0)^m
    \label{eq:M14-expand}
\end{align}
% where since $1/4\ll 1$, we used $\prod_{i=0}^m(-1/4-i) \approx {1\over 4} (-1)^{m+1} m!$. 
Since $M_0$ is positive semi-definite and its largest eigenvalue is one, the sum in \eqref{eq:M14-expand} can be truncated after $q\sim O(1)$ terms. 
% \nd{should we change to $M/(m_{max}+\xi)$ for a small $\xi\ll1$ to argue for truncating the sum? (since technically we need all eigenvalues smaller than 1)}
The first $q$ terms of 
\eqref{eq:M14-expand} can be implemented as a $q$ layer GCN with aggregation function $f(M) = I-M_0$ and residual connections.
We choose $q$ to be as small as $1$ or $2$, as larger $q$ may actually slow down the optimization. 
% \nd{move following to appendix?}
Note that computing $f(M)^q\theta $ is $O(qn^2)$ because we do not need to first compute $f(M)^q$ (which is $O(qn^3)$) and instead use $\vv_{i+1}f(M)\vv_i$ ($O(n^2)$) $q$ times with $\vv_1 = \theta$. 
% \nd{discuss architecture details.}

Lastly, to evaluate $M_0$ we need to estimate the leading eigenvalue $m_{max}$. 
% \nd{Since $1/4$ is much smaller than one, $\prod_{i=0}^m(-1/4-i) \approx (-1)^m m!$ and we can further simplify?} 
We can use a similar expansion for approximating $m_{max}$. 
Given any vector $\vv \in \R^n$ and using the spectral expansion we have 
\begin{align}
    M^q \vv &= \sum_i m_i^q  (\psi_i^T \vv)\psi_i
\end{align}
Since $M$ is positive semi-definite, for $q>1$ the leading eigenvector $\psi_{max}$ quickly dominates the sum and we have $M^q \vv \approx m_{max}^q (\psi_{max}\vv)\psi_{max} $.
Additionally, using the generalized Perron-Frobenius theorem (\cite{berman1994nonnegative}) \nd{cite - check this one}, the components of the leading eigenvector $\psi_{max}$ should be mostly positive. 
Therefore, a good choice for $\vv$, which may be close to the actual $\psi_{max}$, is $\vv = \mathbf{1}/\sqrt{n}$, where $\mathbf{1}= (1,\dots, 1)$.
This yields 
\begin{align}
    \mathbf{1}^T M^p \mathbf{1} &\approx m_{max}^p (\psi_i^T \mathbf{1})^2, & 
    m_{max}^{p-1} &\approx \frac{\mathbf{1}^T M^p \mathbf{1}}{\mathbf{1}^T M \mathbf{1}}
\end{align}
% Note, this approximation is by no means precise as the deviation of the denominator from $m_{max}$ can be significant. 
This is a crude approximation, but it serves our goal by being computationally efficient. 
Note that, while computing $M^q$ is $O(qn^3)$, because $M\mathbf{1}$ is $O(n^2)$, computing $M^q\mathbf{1}$ is $O(qn^2)$.  
Therefore, we choose $p=2$ and write 
\begin{align}
    m_{max} \approx \frac{\mathbf{1}^TM^2 \mathbf{1}}{\mathbf{1}^T M \mathbf{1}} = \frac{\sum_{ij} M_{ij}^2}{\sum_{ij} M_{ij}} 
    \label{eq:m-max-approx-D2}
\end{align}
It is worth noting that if we think of $M$ as the weighted adjacency matrix of a graph with $n$ vertices, the vector component $D_i = [M\mathbf{1}]_i= \sum_jM_{ij} $ is the weighted degree of node $i$.
Hence \eqref{eq:m-max-approx-D2} states $M/m_{max} \approx\pa{\sum_i D_i/ \|D\|^2} M $. 
This is reminiscent of the graph diffusion operator $D^{-1} M$ and $D^{-1/2}MD^{-1/2}$ which are used as the aggregation functions in GCN (here $D_{ij} = D_i \delta_{ij}$ is the diagonal degree matrix).

\Eqref{eq:dLdt-Neural} decomposes the rate of convergence into a part $M$ arising from the loss function and a part $K$ capturing the effect of the neural architecture. 
To understand the interplay between these two matrices, we will first work out the toy example of convex optimization.

\section{experiments}

\textbf{Results of Kuramoto Model.}
Figure \ref{fig:Kuramoto_lattice} shows the results of Kuramoto model on a square lattice.  
Additional results on  circle graph, and tree graph can be found in Appendix \ref{app:exp}.  
Figure \ref{fig:Kuramoto_lattice} (a) shows that NR with one-layer GCN (GCN-1) and GCN with residual connection (RGCN-1) achieves significant speedup. 
In particular, we found $3.6 \pm .5$ speed improvement for the lattice, $6.1 \pm .1$ for the circle graph and $2.7 \pm .3$ for tree graphs. 
We also experimented with two layer (GCN/RGCN-2) and three layer (GCN/RGCN-3) GCNs.  
As expected, the overhead of deeper GCN models slows down optimization and offsets the NR speedup gains.
Figure \ref{fig:Kuramoto_lattice} (b) visualizes the evolution of the oscillator phase $\phi_i$ on a square lattice over iterations. 
We can see that even though different reparametrization models reach the same loss value, the final solutions are quite different. 
The linear version (without NR) arrives at the final solution smoothly, while GCN models form dense clusters at the initial steps and reach an organized state before $100$ steps.  
To quantify the level of synchronization, we measure a quantity $\rho$ known as the ``global order parameter'' (\cite{sarkar2021phase}):
$
    \rho = \frac{1}{N} \left|\sum_{j} e^{i\phi_j} \right| 
    % \label{eq:Order-paramter}
$.
Figure \ref{fig:Kuramoto_lattice} (c) shows the convergence of the global order parameter over time. We can see that one-layer GCN and RGCN gives the highest amount of acceleration, driving the system to synchronization.
\out{
\begin{figure}%[t!]
    \centering
    % a\hfill b\hfill c\hfill .
    \includegraphics[width=\linewidth,
    % trim=0 0 0 .5in, clip
    ]{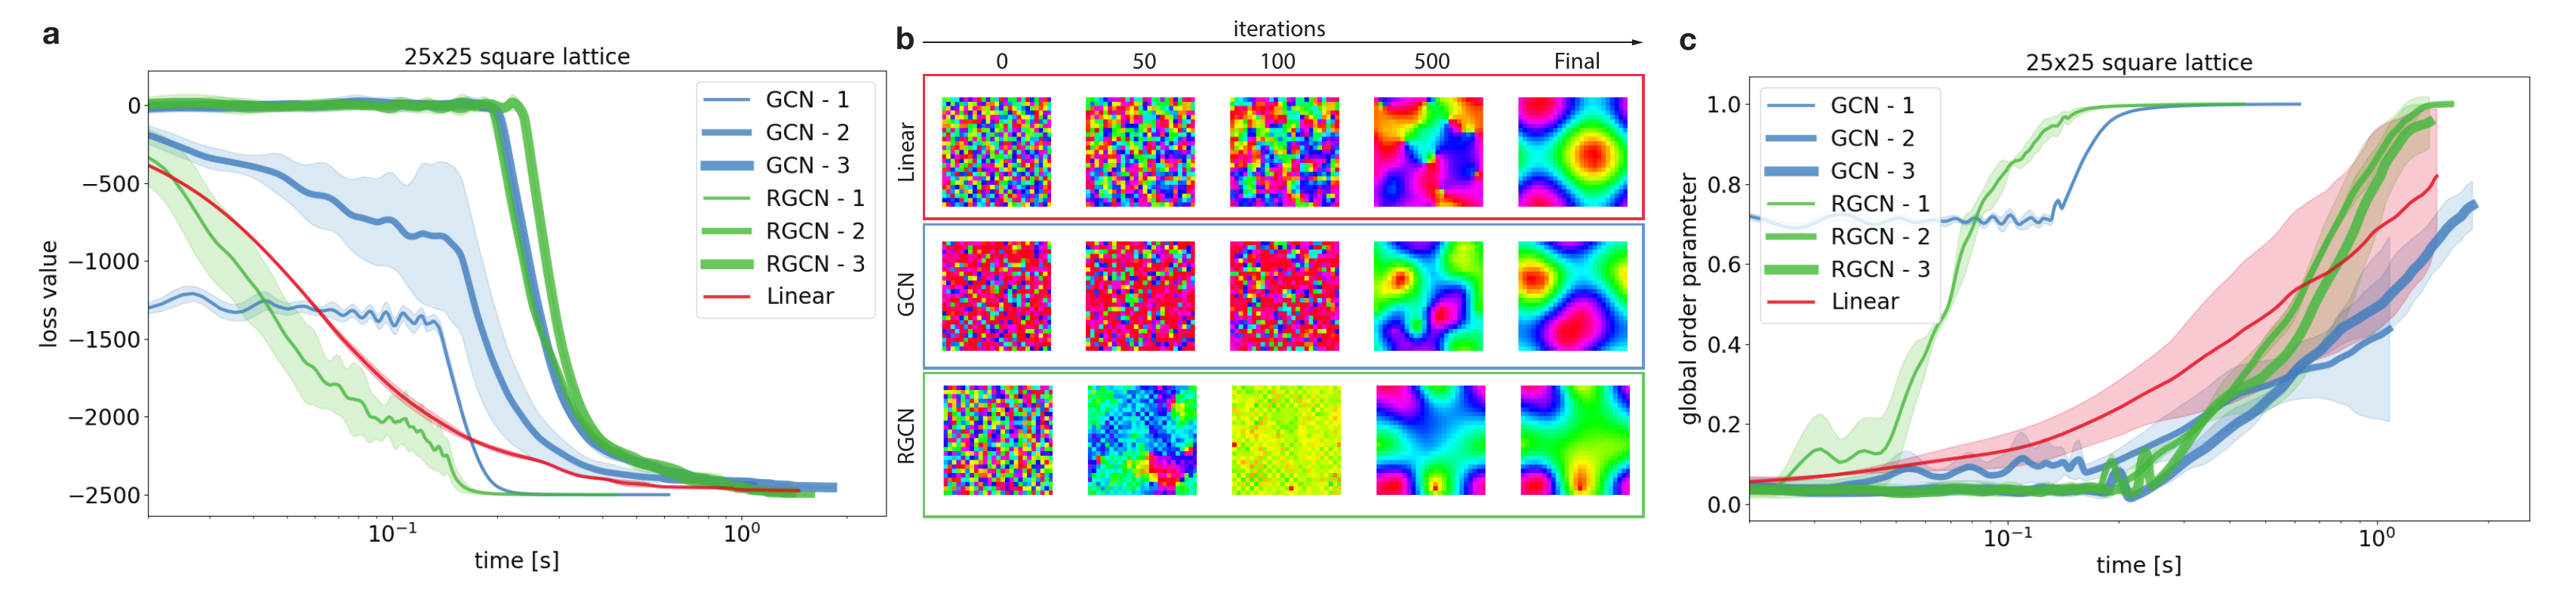}
    \caption{Optimizing Kuramoto model on a $25\times 25$ square lattice (a) Loss over run time in seconds for different methods.  (b) Evolution of the phase variables  over iterations. (c) Level of synchronization, measured by global order parameter over time. Neural reparameterization with GCN achieves the highest speedup.}
    \label{fig:Kuramoto_lattice}
\end{figure}
}

\begin{figure*}[ht!]
\vskip 0.2in
\begin{center}
\centerline{ \includegraphics[width=\linewidth,
    trim=0 0 0 .5in, %clip
    ]{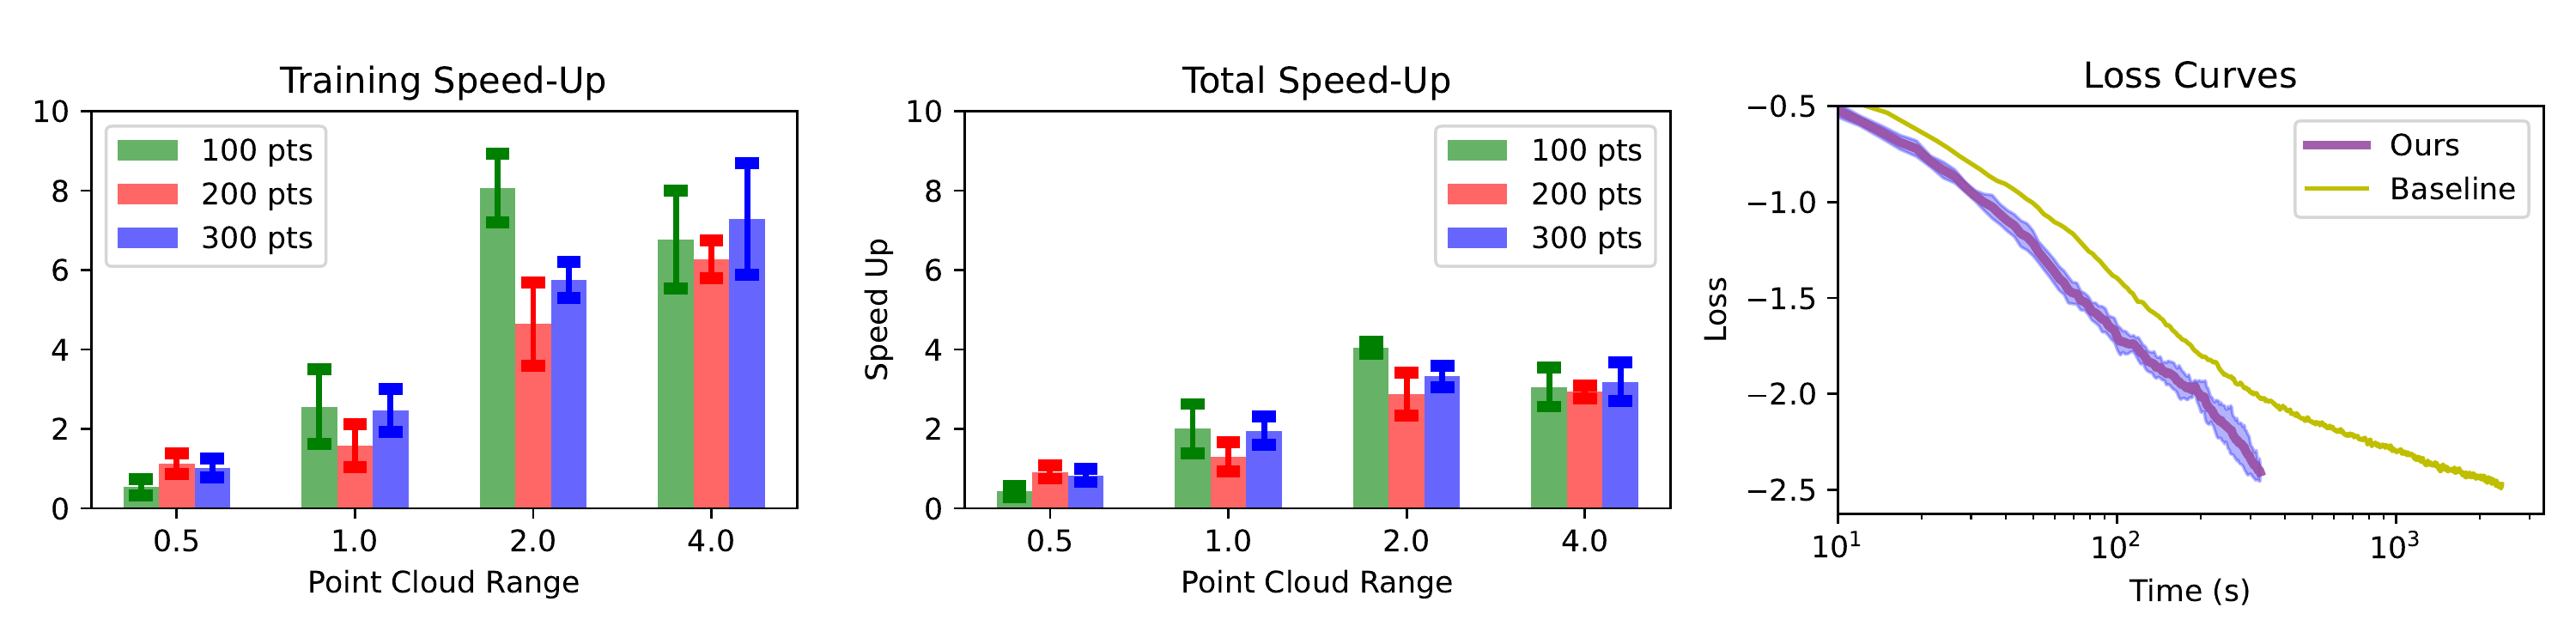}
}
    \caption{{Speedup:} a,b) Training and total time speedup; c) GCN speeds up convergence.}
    \label{fig:GCN_1L_speedup}
\end{center}
\vskip -0.2in
\end{figure*}

\begin{figure}[h]

%  \vskip 0.2in
\begin{center}
\centerline{ 
    \includegraphics[scale=0.35]{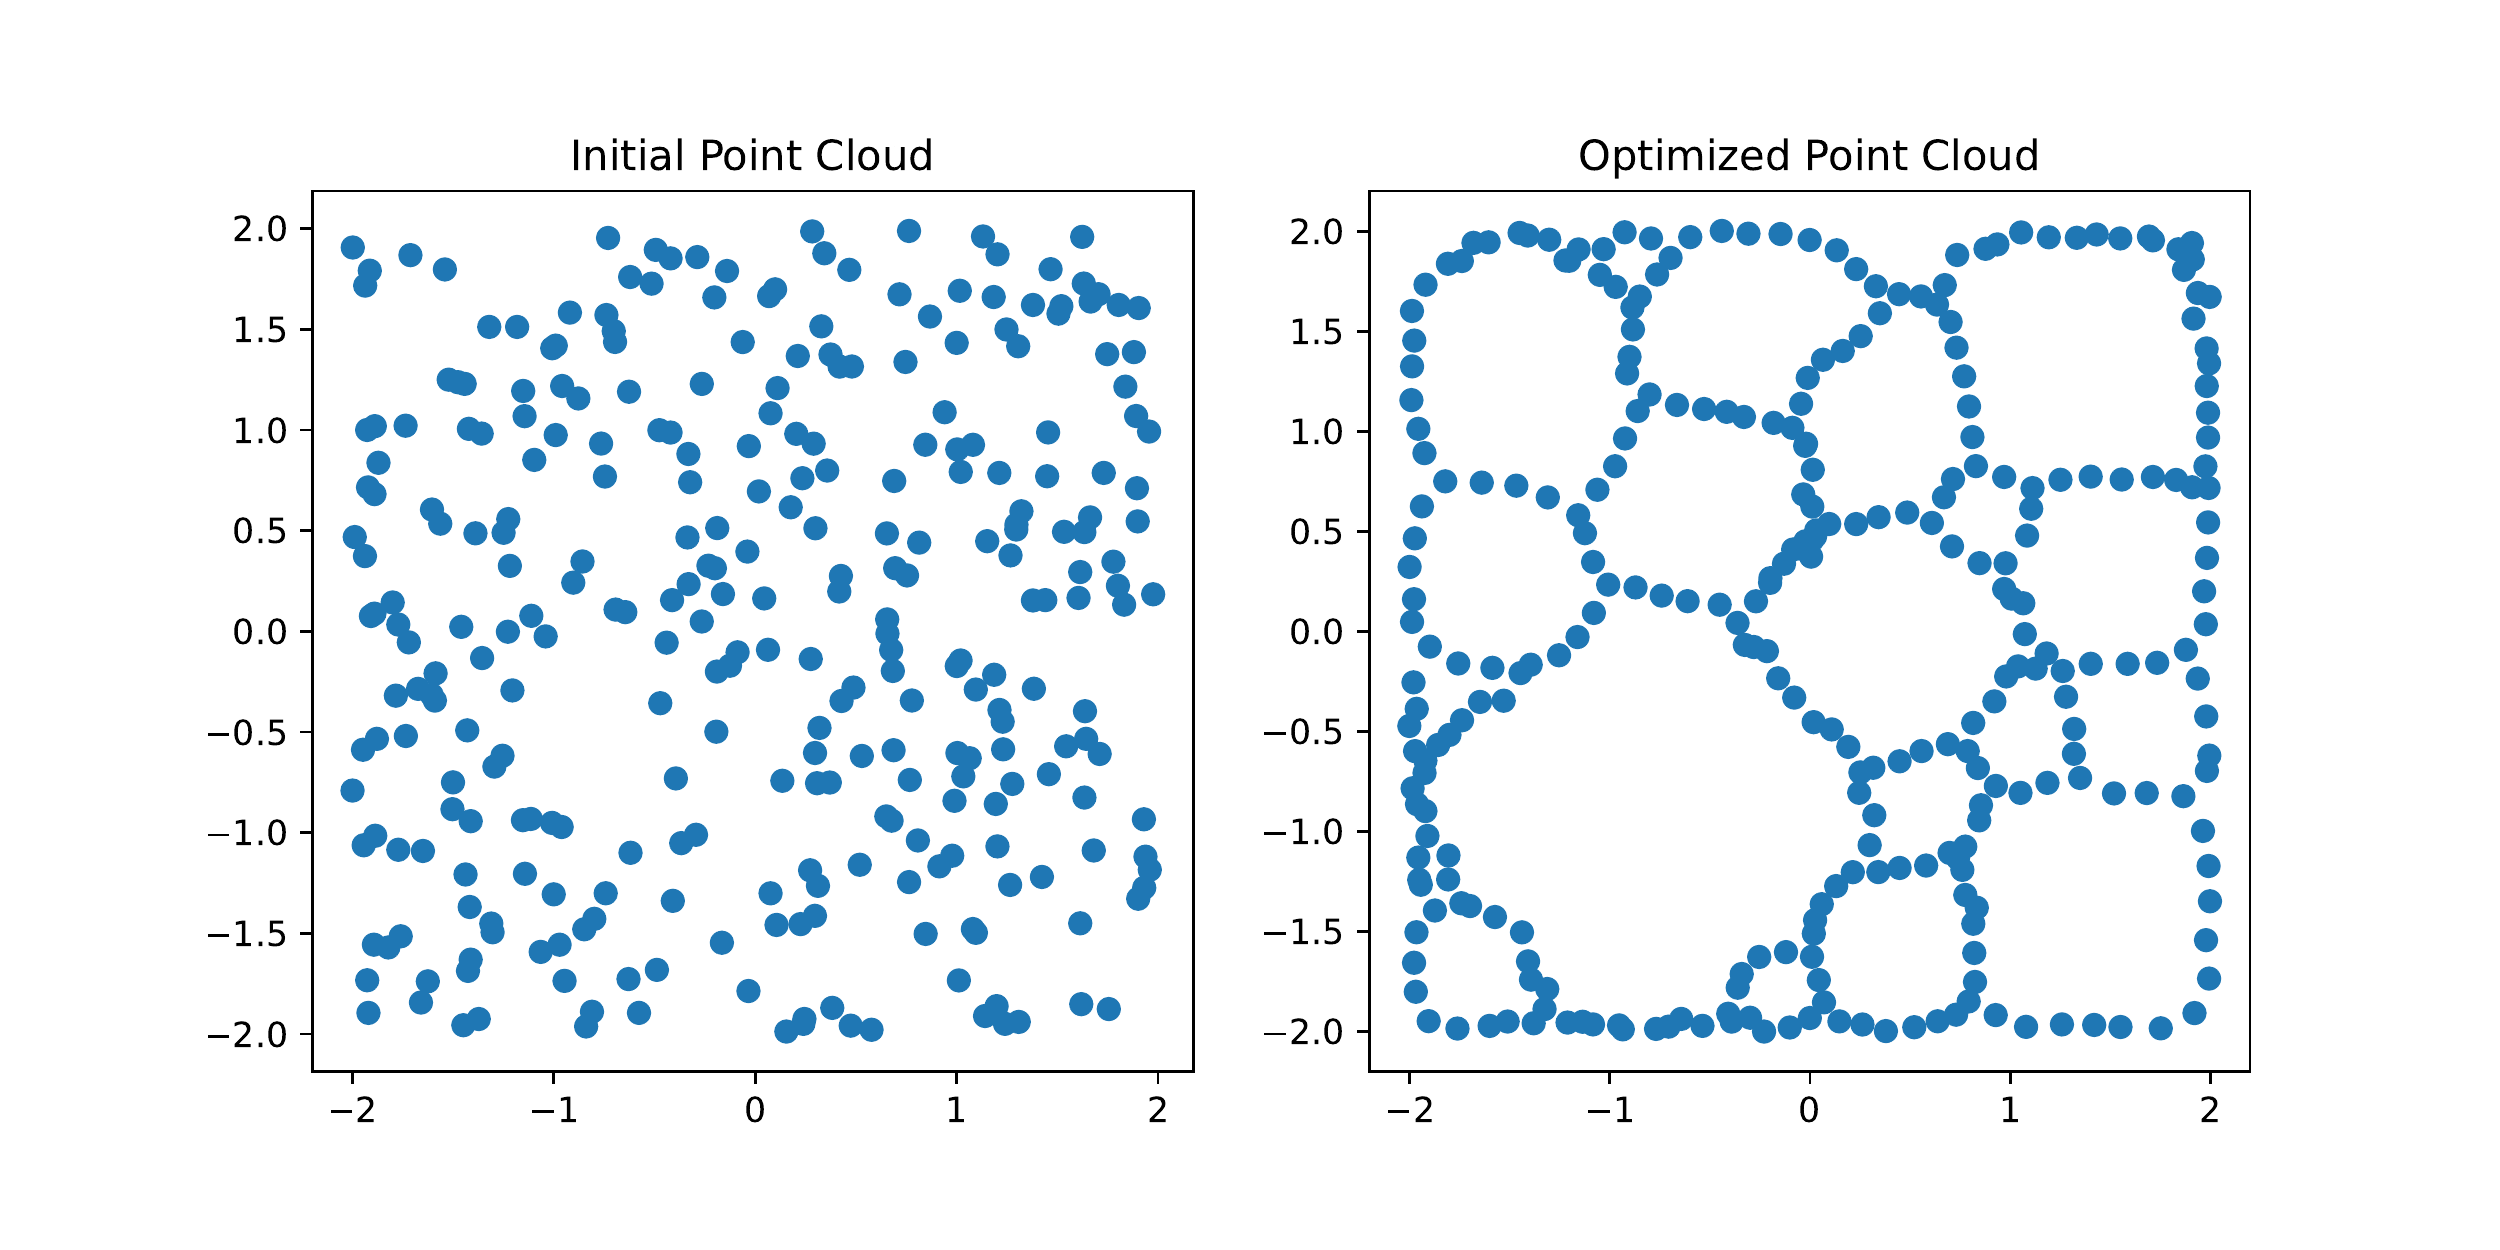}
    \includegraphics[width=.5\linewidth]{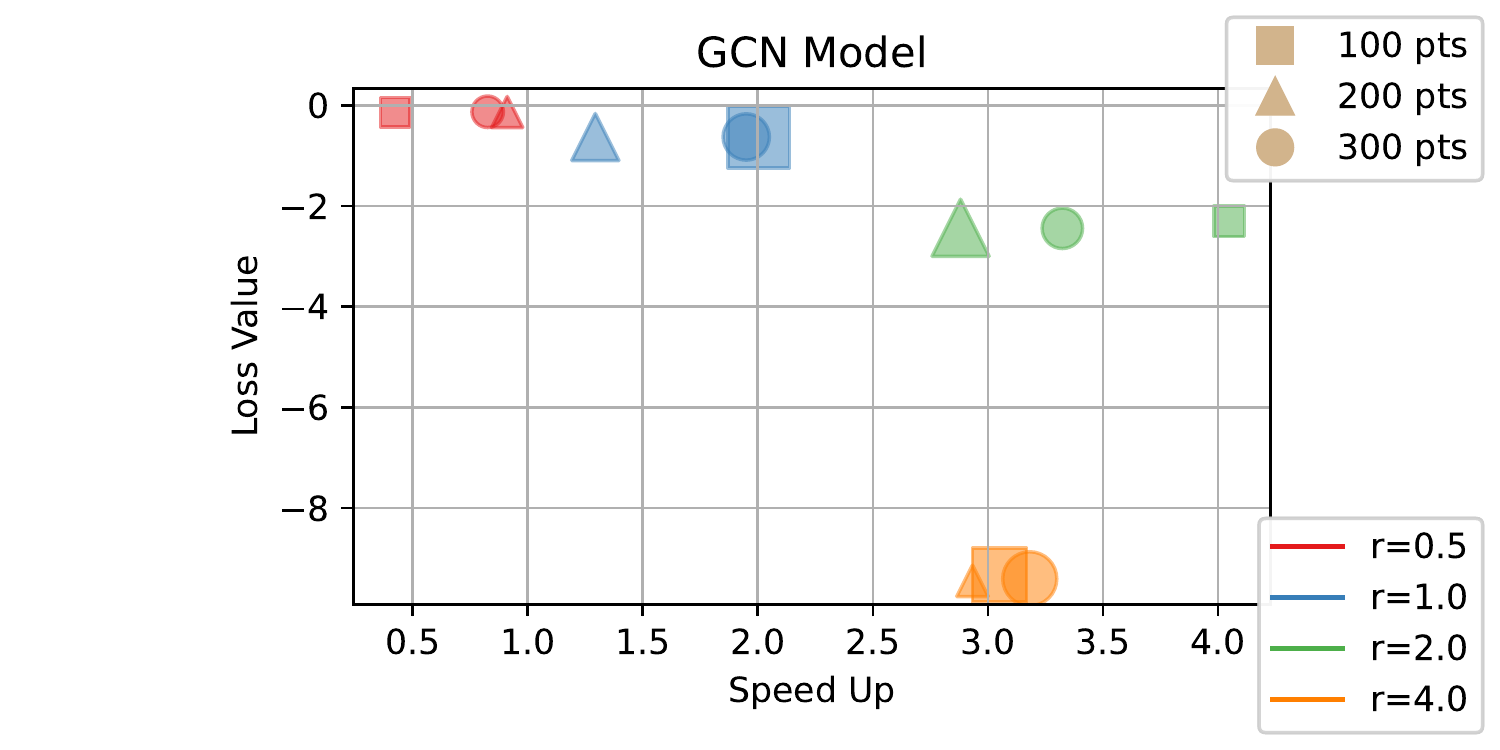}
}
 \caption{Left: Initial random point cloud and optimized point cloud. Right: Loss vs speed-up of GCN model. The converged loss value is determined by point cloud range only, while the speed-up is affected by both point cloud range and size.}
  \label{fig:loss_vs_speedup}
    \end{center}
\vskip -0.2in
\end{figure}

%\begin{figure}[ht]
%    \centering
    % a\hfill b\hfill c\hfill .
%    \includegraphics[width=\linewidth,
    % trim=0 0 0 .5in, clip
 %   ]{figures/Hopf-Kuramoto/HK-1.pdf}
%    \caption{Hopf-Kuramoto model on a square lattice ($50\times 50$). a, b) Speedup in the final loss value difference function, wherein case a) both models converged b) linear model converged, and the GCN model achieved the same loss value. Points color correspond to the regions of the phase diagram (c). }
%    \label{fig:hopf_kuramoto}
%\end{figure}

% \out{
% \begin{figure}
%     \centering
%     \includegraphics[width=.45\linewidth]{figures/625_circle_op_it_loss_alpha0_lw.pdf}
%     \includegraphics[width=.45\linewidth]{figures/625_circle_op_it_loss_alpha0_lw.pdf}
%     \caption{Caption}
%     \label{fig:my_label}
% \end{figure}

% \begin{figure}[!htb]
%     \centering
%     \includegraphics[width= 1\linewidth,trim=0 0 0 0,clip]{figures/sync_1.pdf}
%     \caption{a) disorganized b) organized phase   }
%     \label{fig:sync}
% \end{figure}

% \begin{figure}[!htb]
%     \centering
%     \includegraphics[width= 1\linewidth,trim=0 0 0 0,clip]{figures/speedup_2d.pdf}
%     \caption{Speedup 2d lattice }
%     \label{fig:HK speedup}
% \end{figure}

% }%%% 

\textbf{Results of Hopf-Kuramoto Model.} We report the comparison of NR models on synchronizing Hopf-Kuramoto dynamics.
According to the \citet{lauter2015pattern} paper, we identify two different main patterns on the phase diagram Fig. \ref{fig:HK-pattern}(b): ordered (small $s_2/c$, smooth patterns) and disordered (large $s_2/c$, noisy) phases.
In all experiments we use the same lattice size $50 \times 50$, with the the same stopping criteria ($10$ patience steps and $10^{-10}$ loss error limit) and switch between the Linear and GCN model after $100$ iteration steps.
Fig. \ref{fig:hopf_kuramoto} (a) shows the loss at convergence versus the speedup.  We compare different GCN models and observe that GCN with $A^2$ as the propagation rule achieves the highest speedup. 
Also, we can see that we have different speedups in each region, especially in the disordered phases. 
Furthermore, we observed that the Linear and GCN models converge into a different minimum state in a few cases. However, the patterns remain the same. (b) shows how the level of ordering changes region by region. If the global order parameter is closer to $0$, we have more of a disordered phase while the parameter is closer to $1$, meaning it is a more organized pattern.

We know that running dynamics in a large lattice are computationally expensive, especially close to the phase transition points where difficult to separate the slow and fast modes.

\subsection{Persistent homology}
Persistent homology \citet{edelsbrunner2008persistent} is an algebraic tool for measuring topological features of shapes and functions. Recently, it has found many applications in machine learning \cite{hofer2019connectivity, gabrielsson2020topology, birdal2021intrinsic}. Persistent homology is computable with linear algebra and robust to perturbation of input data \citep{otter2017roadmap}, see more details in Appendix \ref{app:homology}.

An example application of persistent homology is point cloud optimization \cite{gabrielsson2020topology, carriere2021optimizing}. As shown in Fig. \ref{fig:loss_vs_speedup} left, given a random point cloud $\vw$ that lacks any observable characteristics, we aim to produce persistent homological features by optimizing the position of data points.
\begin{eqnarray}
\L(\vw) = -\sum_{p\in D}\| p -\pi_{\Delta} (p)\|^2_\infty + \sum_{i=1}^n \|\vw_i-r\|^2
\label{eqn:opt_persisten}
\end{eqnarray}
where $p\in D = \{(b_i,d_i)\}_{i\in I_k}$ denotes the homological features in the the persistence diagram $D$, consisting of all the pairs of birth $b_i$ and death $d_i$ filtration values of the set of k-dimensional homological features $I_k$. $\pi_{\Delta}$ is the projection onto the diagonal $\Delta$ and $\sum_i d(\phi_i,S)$ constrains the points within the a square centered at the origin with length $2r$ (denote $r$ as range of the point cloud).

\cite{carriere2021optimizing} optimizes the point cloud positions directly with gradient-based optimization. We will refer theirs as the baseline linear model. 
In contrast, we integrate GCN and reparameterize the point cloud positions, and will refer ours as the GCN model.

\textbf{Implementation.}
To measure the speed-up of GCN model, we used the same Gudhi library for computing persistence diagram as \cite{gabrielsson2020topology, carriere2021optimizing}. The  runtime of learning persistent homology is dominated by computing persistence diagram in every iteration, which has the time complexity of $O(n^3)$. % where $n$ is the point cloud size. 
% Under this condition, 
Thus, the runtime per iteration for GCN model and linear model are very similar, and we demonstrate that the GCN model can reduce convergence time by a factor of $\sim4$. 
We ran the experiments for point cloud of $100$,$200$,$300$ points, with ranges of $0.5$,$1.0$,$2.0$,$4.0$. 
The hyperparameters of the GCN model are kept constant, including network dimensions. 
The result for each setting is averaged from 5 consecutive runs.

\textbf{Persistent Homology Results.}
Fig. \ref{fig:loss_vs_speedup} right shows that the speedup of the GCN model is related to point cloud density. 
Training converges faster as the point cloud becomes more sparse, but the speedup gain saturates as point cloud density decreases. 
On the other hand, time required for initial point cloud fitting increases significantly with the range of point cloud. 
Consequently, the overall speedup peaks when the range of point cloud is around 4 times larger than what is used be in \cite{gabrielsson2020topology, carriere2021optimizing}, which spans over an area 16 times larger. 
Further increase in point cloud range causes the speedup to drop as the extra time of initial point cloud fitting outweighs the reduced training time. 
The loss curve plot in Fig. \ref{fig:GCN_1L_speedup} shows the convergence of training loss of the GCN model and the baseline model in one of the settings when GCN is performing well.
Fig. \ref{fig:loss_vs_speedup} shows the initial random point cloud and the output from the GCN model. 
In the Appendix  \ref{app:homology}, we included the results of GCN model hyperparameter search and a runtime comparison of the GCN model under all experiment settings.

\out{
\begin{figure}
    \centering
    \includegraphics[width=.45\linewidth]{figures/625_circle_op_it_loss_alpha0_lw.pdf}
    \includegraphics[width=.45\linewidth]{figures/625_circle_op_it_loss_alpha0_lw.pdf}
    \caption{Caption}
    \label{fig:my_label}
\end{figure}

\begin{figure}[!htb]
    \centering
    \includegraphics[width= 1\linewidth,trim=0 0 0 0,clip]{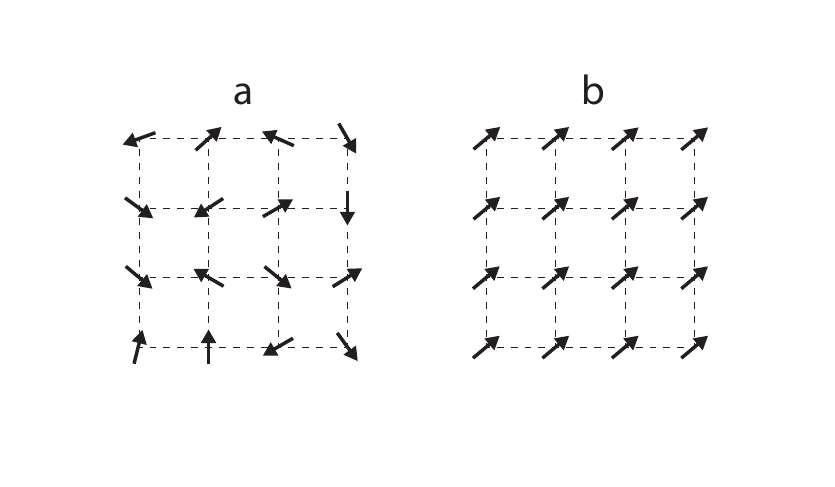}
    \caption{a) disorganized b) organized phase   }
    \label{fig:sync}
\end{figure}

\begin{figure}[!htb]
    \centering
    \includegraphics[width= 1\linewidth,trim=0 0 0 0,clip]{figures/speedup_2d.pdf}
    \caption{Speedup 2d lattice }
    \label{fig:HK speedup}
\end{figure}

}%%% 
